# Supplementary material for: Anomalous thermal expansion and chiral phonons in BiB$_{3}$O$_{6}$
Source: arXiv:1902.07498 ancillary file (2019-07-03)
Supplement: Supplementary file 1 [file Supplemental_Material.pdf]

# Anomalous thermal expansion and chiral phonons in $BiB_3O_6$: Supplemental Material

Carl P. Romao[1,2,*]

[1]*Department of Chemistry, University of Oxford, Inorganic Chemistry Laboratory, South Parks Road, Oxford OX1 3QR, UK*

[2]*Section for Solid State and Theoretical Inorganic Chemistry, Institute of Inorganic Chemistry, University of Tübingen, Auf der Morgenstelle 18, D-72076 Tübingen, Germany*

(Dated: May 23, 2019)

## COMPUTATIONAL METHODS, ELASTIC TENSORS, AND THERMAL EXPANSION TENSORS

Initially, calculations were performed using the projector-augmented wave (PAW) method [1] and the local density approximation (LDA) to the exchange–correlation functional [2]. The LDA is known to give generally accurate phonon energies for inorganic materials [3]. PAW datasets from the ABINIT library were used as received [4]. A $4\times4\times4$ Monkhorst–Pack grid [5] in **k**-space and a 32 Ha plane-wave energy cut-off were chosen by convergence studies (the criterion used was convergence of the pressure within 1 %). Preliminary validation was performed by comparison to the experimental elastic tensor, extrapolated to 0 K (Table I) [6]; calculations using the LDA were found to be in decent agreement with experiment in this regard. However, as shown in Table II, the calculated CTEs deviated enormously from the experimental values, as large positive thermal expansion was predicted in all directions.

The dispersion correction of Grimme to the exchange–correlation functional with Becke–

TABLE I. Calculated elements of the elastic stiffness tensor (in GPa) of $\alpha$-$BiB_3O_6$, compared to the experimental result of Ref. 6.

| Element | LDA | PBE GGA vdw-D3(BJ) | Experimental [6] |
|---|---|---|---|
| $c_{11}$ | 253.7 | 205.3 | 170.3 |
| $c_{22}$ | 38.8 | 72.9 | 56.5 |
| $c_{33}$ | 127.8 | 165.0 | 215.7 |
| $c_{44}$ | 13.7 | 22.3 | 24.4 |
| $c_{55}$ | 92.2 | 88.0 | 79.8 |
| $c_{66}$ | 75.4 | 69.4 | 69.3 |
| $c_{12}$ | 63.1 | 64.3 | 78.9 |
| $c_{13}$ | 74.0 | 77.9 | 61.8 |
| $c_{23}$ | 3.7 | 18.0 | 15.1 |
| $c_{15}$ | −66.9 | −52.2 | −51.6 |
| $c_{25}$ | 14.7 | 5.9 | −4.4 |
| $c_{35}$ | −56.6 | −41.5 | −74.9 |
| $c_{46}$ | −4.8 | −9.1 | −18.9 |

TABLE II. Calculated elements of the thermal expansion tensor at 300 K (in $10^{-6}$ $K^{-1}$) of α-$BiB_3O_6$, compared to the experimental result of Ref. 7.

| Element | LDA | PBE GGA vdw-D3(BJ) | Experimental [7] |
|---|---|---|---|
| $\alpha_{11}$ | 24.6 | −7.5 | −25.6 |
| $\alpha_{22}$ | 118.4 | 8.1 | 50.4 |
| $\alpha_{33}$ | 35.4 | 5.2 | 7.7 |
| $\alpha_{13}$ | 17.7 | −10.2 | −5.33 |

Johnson damping (known as "vdw-D3(BJ)") [8, 9] was then introduced to the calculations in an attempt to increase their accuracy; for compatibility optimized norm-conserving Vanderbilt pseudopotentials [10] and the Perdew–Burke–Ernzerhof general gradient approximation [11] (PBE GGA) to the exchange–correlation functional were also employed. These calculations used pseudoptentials from the Abinit library, a $4 \times 4 \times 4$ Monkhorst–Pack grid [5] in **k**-space, a 34 Ha plane-wave energy cut-off, and a $10^{-10}$ Ha cutoff for contributions of pairs of atoms to the dispersion potential. An example input file for a calculation of the phonon band structure is included as part of this Supplemental Material.

The calculated elastic tensor replicated the experimental one with generally improved accuracy compared to the LDA case (Table I). The calculated CTE tensor was able to qualitatively reproduce the thermal expansion behaviour, unlike in the LDA case. However, the agreement was somewhat poor as the thermal expansion in the **ab** plane was significantly underestimated. To test the sensitivity of the calculated CTE to specific DFT inputs, the calculations were repeated using the vdw-D3 dispersion correction without Becke–Johnson damping [8], and with pseudopotentials provided by D. R. Hamman [12]. Varying the specific form of the dispersion correction and the pseudopotential set used did not result in improvements in the accuracy of the calculated CTE and therefore the results presented in the main body of this work are those obtained using PBE GGA vdw-D3(BJ).

Comparison of the calculated CTE tensors therefore shows that the anomalous thermal expansion of α-$BiB_3O_6$ is influenced significantly by dispersion interactions. While the form of the exchange–correlation functional also changed from LDA to PBE GGA; this will, on its own, increase phonon energies and decrease stiffness and therefore increase the magnitude of the calculated CTE rather than decrease it [3]. Since thermal expansion is related to the

third-order and higher derivatives of the potential energy surface for atomic displacement, it follows that it is highly sensitive to dispersive interactions. The vdw-D3 dispersion correction incorporates the atomic coordination number in its parametrization; this parametrization is based on *ab intio* calculations of the polarizabilities of binary hydrides [8]. As the α-$BiB_3O_6$ structure contains tetracoordinate bismuth and boron atoms, the dispersion coefficients for these atoms must be obtained from extrapolation rather than interpolation, and therefore some degradation of their accuracy can be expected.

## MODE GRÜNEISEN PARAMETERS WITHOUT DISPERSION CORRECTION

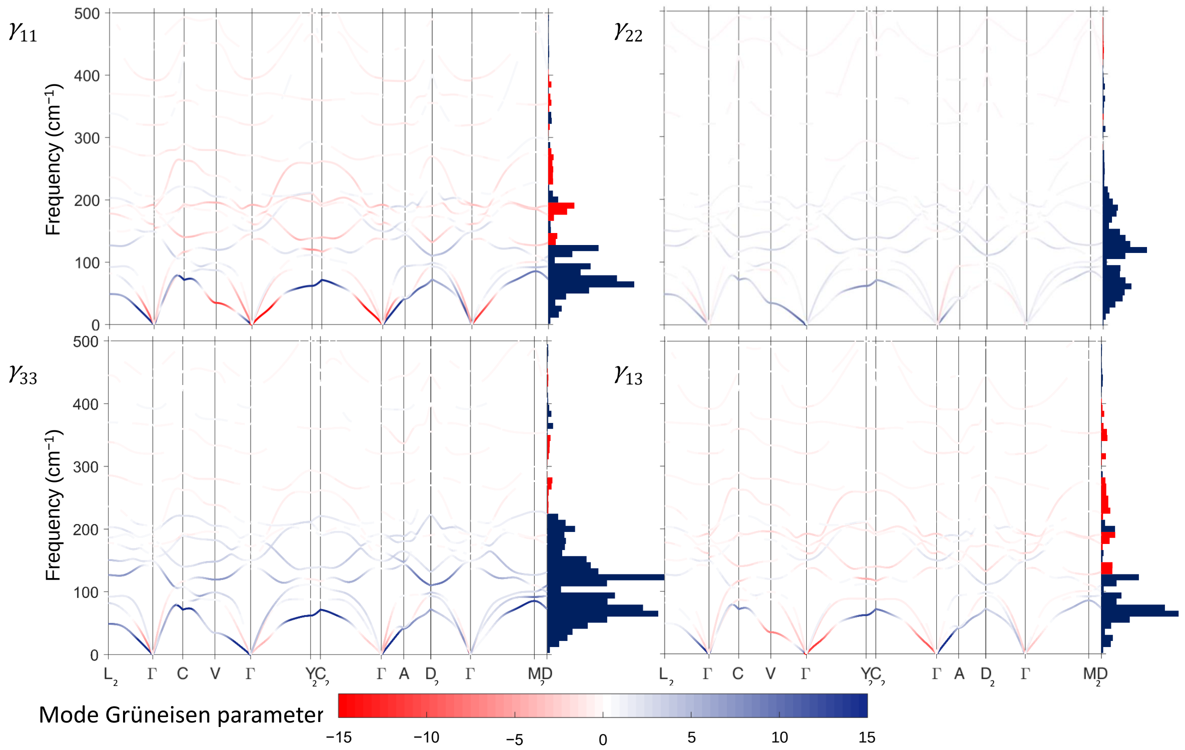


FIG. 1. Phonon band structure of α-$BiB_3O_6$, calculated using the LDA and without a dispersion correction to the exchange–correlation functional. Bands are coloured according to their directional mode Grüneisen parameters ($\gamma_{ij,n,\mathbf{k}}$) calculated using the method of Ref. 13. Phonons with energies greater than 500 $cm^{-1}$ do not contribute significantly to thermal expansion and are not shown. The density of states ($\rho$), weighted by the Grüneisen parameters as $\sum_{\mathbf{k}} \rho_{\mathbf{k}}(\omega)\gamma_{ij,\mathbf{k}}(\omega)$, is shown as a histogram at the right of each plot, with positive values coloured in blue and negative values in red. Special points in the Brillouin zone were selected following Ref. 14.

## PHONON POLARIZATIONS

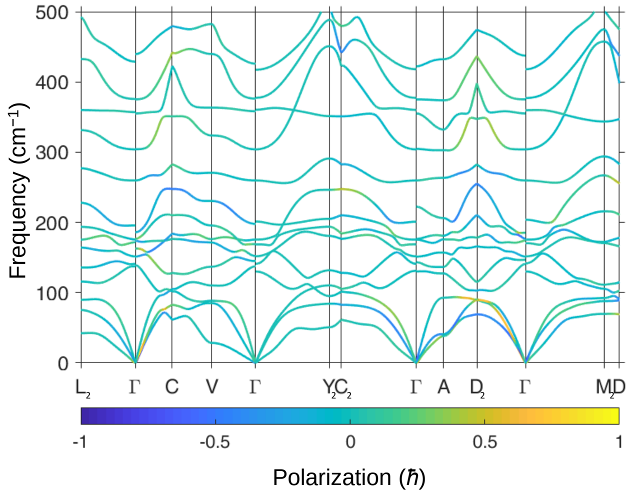


FIG. 2. Phonon band structure of α-$BiB_3O_6$, with bands coloured according to their circular polarizations along **x** ($S_{11}$). A polarization of $\hbar$ corresponds to a fully right-polarized phonon [15]. Special points in the Brillouin zone were selected following Ref. 14.

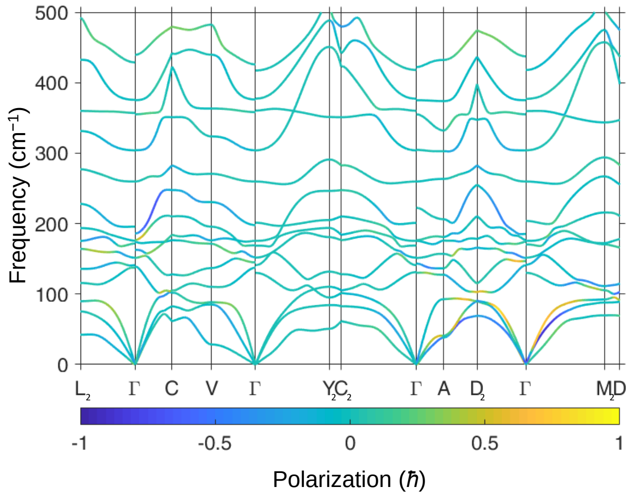


FIG. 3. Phonon band structure of α-$BiB_3O_6$, with bands coloured according to their circular polarizations along **z** ($S_{33}$). A polarization of $\hbar$ corresponds to a fully right-polarized phonon [15]. Special points in the Brillouin zone were selected following Ref. 14.

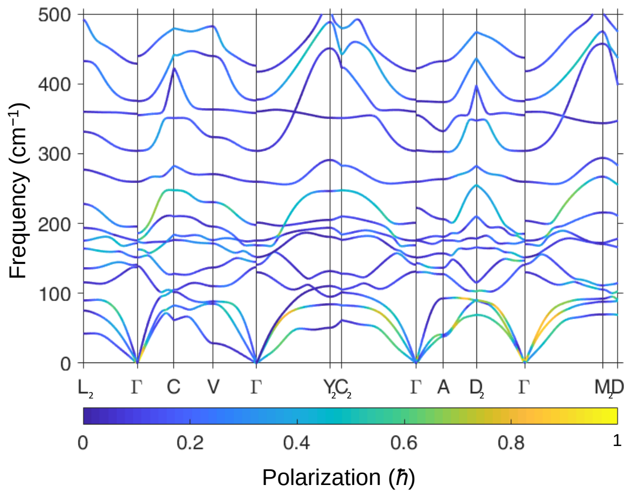


FIG. 4. Phonon band structure of α-$BiB_3O_6$, with bands coloured according to the magnitude of their circular polarization (*i.e.,* $||\mathbf{S}||$). A polarization of $\hbar$ corresponds to a fully right-polarized phonon [15]. Special points in the Brillouin zone were selected following Ref. 14.

* carl.romao@mnf.uni-tuebingen.de

[1] M. Torrent, F. Jollet, F. Bottin, G. Zérah, and X. Gonze, Implementation of the projector augmented-wave method in the ABINIT code: Application to the study of iron under pressure, Comp. Mater. Sci. **42**, 337 (2008).

[2] W. Kohn and L. J. Sham, Self-consistent equations including exchange and correlation effects, Phys. Rev. **140**, A1133 (1965).

[3] L. He, F. Liu, G. Hautier, M. J. Oliveira, M. A. Marques, F. D. Vila, J. Rehr, G.-M. Rignanese, and A. Zhou, Accuracy of generalized gradient approximation functionals for density-functional perturbation theory calculations, Phys. Rev. B **89**, 064305 (2014).

[4] psps tables — ABINIT, `https://www.abinit.org/psp-tables`, accessed: 2017-01-20.

[5] H. J. Monkhorst and J. D. Pack, Special points for Brillouin-zone integrations, Phys. Rev. B **13**, 5188 (1976).

[6] L. Kang, X. Jiang, S. Luo, P. Gong, W. Li, X. Wu, Y. Li, X. Li, C. Chen, and Z. Lin, Negative linear compressibility in a crystal of α-$BiB_3O_6$, Sci. Rep. **5**, 13432 (2015).

[7] B. Teng, Z. Wang, H. Jiang, X. Cheng, H. Liu, X. Hu, S. Dong, J. Wang, and Z. Shao,

Anisotropic thermal expansion of $BiB_3O_6$, J. Appl. Phys. **91**, 3618 (2002).

[8] S. Grimme, J. Antony, S. Ehrlich, and H. Krieg, A consistent and accurate ab initio parametrization of density functional dispersion correction (DFT-D) for the 94 elements H-Pu, J. Chem. Phys. **132**, 154104 (2010).

[9] A. D. Becke and E. R. Johnson, A simple effective potential for exchange, J. Chem. Phys. **124**, 221101 (2006).

[10] D. R. Hamann, Optimized norm-conserving Vanderbilt pseudopotentials, Phys. Rev. B **88**, 085117 (2013).

[11] J. P. Perdew, K. Burke, and M. Ernzerhof, Generalized gradient approximation made simple, Phys. Rev. Lett. **77**, 3865 (1996).

[12] SG15 ONCV potentials, `http://www.quantum-simulation.org/potentials/sg15_oncv/`, accessed: 2017-01-20.

[13] C. P. Romao, Anisotropic thermal expansion in flexible materials, Phys. Rev. B **96**, 134113 (2017).

[14] Y. Hinuma, G. Pizzi, Y. Kumagai, F. Oba, and I. Tanaka, Band structure diagram paths based on crystallography, Comp. Mater. Sci. **128**, 140 (2017).

[15] L. Zhang and Q. Niu, Chiral phonons at high-symmetry points in monolayer hexagonal lattices, Phys. Rev. Lett. **115**, 115502 (2015).
